# Supplementary material for: F-coref: Fast, Accurate and Easy to Use Coreference Resolution
Source: arXiv:2209.04280 source file (2022-10-25)
Supplement: Supplementary file 1 [file 08_appendix.tex]

\clearpage
\appendix

\section{Implementation details}
\label{app:implementation}

As mentioned in the paper~(Section~\ref{sec:results}), we train our student model on the teacher predictions that we obtained on the source documents of the Multi-News dataset. Due to \textsc{LingMess} limitations, we omit source documents with more than 4096 tokens from the original dataset. We tokenize each document with Spacy and run the teacher model to predict coreference clusters. 

We implement our model using Pytorch, HuggingFace and the Datasets library. We pre-train the mention scorer of our model on the teacher predicted mentions by optimizing the binary cross-entropy loss for each mentions. We use a learning rate of $3e-04$ for the mention scoring function and $1e-05$ for the distillRoBERTa encoder. Then, we train the full student model on the predicted clusters with $\lambda = 0.25$ using the marginal log likelihood loss, as common in coreference resolution. At this stage, we use a learning rate of $3e-04$ for the antecedent and scorer and a smaller learning rate, $1e-05$, for the mention scorer and encoder in order to finetune them. We further fine-tune our full student model on OntoNotes using a learning rate of $1e-05$ for all parameters.

% The model objective function optimize for each possible mention $q$, the sum of probabilities over the true antecedent $\hat{c}$ of $q$:
% \begin{align*}
% L(q) = \log \sum_{\hat{c} \in \mathcal{C}(q) \cap \textsc{gold}(q)}P(\hat{c} \mid q) 
% \end{align*}

% where $\mathcal{C}(q)$ is the set of all candidate antecedents\footnote{All spans before $q$ that passed some pruning threshold.} with a null antecedent $\varepsilon$. $\textsc{gold}(q)$ is the set of the true antecedents of $q$.
% $P(\hat{c} \mid q)$ is computed as a softmax over $F(c, q)$ scores for $c$ values in $\mathcal{C}(q)$.

% \begin{itemize}
%     \item pytorch and huggingface Implementation
%     \item flatten/split multi-news dataset documents to multiple documents.
%     \item tokenize each doc with spacy
%     \item inference clusters from teacher for each doc
%     \item load the finetune distilroberta encoder, training only the mention scorer of the network while finetune the encoder. lr encoder = 1e-05. lr mention scorer=34-04. dynamic bathing. 
%     \item load the finetune distilroberta and the trained mention scorer, and trin the antecedent scorer. now both encoder + mentions corer lr = 1e-05. antecedent scorer lr=3e-04. the lambda at this stage tune with 0.25.
%     \item fine tune ontonotes with total lr of 1e-05. tune with lambda 0.25

%     train the antecedent scorer function only
% \end{itemize}
